# Supplementary material for: Fast Inference for Augmented Large Language Models
Source: arXiv:2410.18248 source file (2024-10-25)
Supplement: Supplementary file 1 [file appendix.tex]

\section{Appendix}
\label{sec:appendix1}

\begin{theorem*}
Consider a system with unlimited servers, a finite number of requests, and a finite total memory capacity $M_{total}$, where each request $i$ has a known service time $S_i$ and memory consumption $M_i$.  A job may experience an additional delay $D_i$ due to memory constraints.  Assume further that service time and memory use is correlated, so $S_i \geq S_j \rightarrow M_i(t) + M_j(s) \geq M_j(s) + M_j(t)$ for any jobs $i$ and $j$
and any times $s$ and $t$. Then scheduling requests in ascending order of $M_i$ minimizes the total response time. 
\end{theorem*}

We note that while service time and memory consumption may not be universally correlated across all jobs, our assumption is generally true for most pairs of jobs.  Accordingly, scheduling requests in ascending order of $M_i$ is a strong greedy heuristic in practice.  Or course, this greedy approach is most effective when higher memory consumption aligns with longer service times, with only rare exceptions.

\begin{proof}
    
We show that swapping any pair of adjacent requests on the same server, where a higher-memory request precedes a lower-memory one, along with corresponding adjustments on other servers, if necessary, does not increase the total response time.

We define the total response time for request $i$ under schedule $\mathcal{S}$ as $R_i(\mathcal{S}) = W_i(\mathcal{S}) + S_i + D_i(\mathcal{S})$ where $W_i(\mathcal{S})$ is the waiting time, $S_i$ is the service time, and $D_i(\mathcal{S})$ is the additional delay for request $i$ due to memory constraints. Let $M_i$ be the memory consumption of request $i$

The total response time is:
\[
T_{\text{total}} (\mathcal{S}) = \sum_{i} R_i(\mathcal{S}) = \sum_{i} (W_i(\mathcal{S}) + S_i + D_i(\mathcal{S})).
\]

Consider $\mathcal{S}$, a schedule that is not in ascending order of $M_i$. At least one pair of adjacent requests exists where a higher-memory request $i$ precedes a lower-memory request $j = i+1$, i.e., $M_i > M_j$. Let $\mathcal{S^\prime}$ be the schedule obtained by swapping $i$ and $j$.  (Note we use $j = i+1$ for brevity.)

Our goal is to show that $\mathcal{S^\prime}$ reduces (or does not increase) total response time. Let $\Delta T_{\text{total}}$ be the change in total response time due to swapping $i$ and $j$ (between $\mathcal{S}$ and $\mathcal{S^\prime}$):
%{\bf MM: Why are only $i$ and $j$ affected?}

\[
\Delta T_{\text{total}} = T_{\text{total}} (\mathcal{S^\prime}) - T_{\text{total}} (\mathcal{S}) = \sum_{i} \Delta R_i,
%(R_i^{\text{after}} + R_j^{\text{after}}) - (R_i^{\text{before}} + R_j^{\text{before}})
\]
where \( \Delta R_i = R_i(\mathcal{S^\prime}) - R_i(\mathcal{S})\).
%Where $$R_x^{\text{before/after}} = W_x^{\text{before/after}} + S_x + D_x^{\text{before/after}} \quad \text{for} \, x \in \{i, j\}$$

\textbf{Changes in $\Delta R_i$ due to $i$ and $j$.}
For $i$ and $j$, the swap only affects their waiting times and additional delays while service times remain the same. In particular, the waiting time for the request $i$ increases by $S_j$.
\[
W_i({\mathcal{S^\prime}}) = W_i({\mathcal{S}}) + S_j.
\]

The waiting time for the request $j$ decreases by $S_i$.
\[
W_j({\mathcal{S^\prime}}) = W_j({\mathcal{S}}) - S_i.
\]

\textbf{Total change for $i$ and $j$:}

\begin{align*}
 = &\left[ (W_i({\mathcal{S}}) + S_j) + S_i + D_i({\mathcal{S^\prime}}) \right. \\
&\left. + (W_j({\mathcal{S}}) - S_i) + S_j + D_j({\mathcal{S^\prime}}) \right] \\
&- \left[ W_i({\mathcal{S}}) + S_i + D_i({\mathcal{S}}) + W_j({\mathcal{S}}) + S_j + D_j({\mathcal{S}}) \right] \\
& = \left[ S_j - S_i + D_i({\mathcal{S^\prime}}) + D_j({\mathcal{S^\prime}}) - D_i({\mathcal{S}}) - D_j({\mathcal{S}}) \right] \\
&= \Delta S + \Delta D_i + \Delta D_j.
\end{align*}

Now consider \textbf{$\Delta D_i + \Delta D_j$:} 
After swapping, with $j$ processed before $i$, the cumulative memory consumption, which is the total memory used by all running requests (as requests complete, they free up memory), is lower when processing $j$. Thus, the additional delays $D_j({\mathcal{S^\prime}})$ and $D_i({\mathcal{S^\prime}})$ may be reduced or removed.

\[
D_i({\mathcal{S^\prime}}) \leq D_i({\mathcal{S}}),
\]
\[
D_j({\mathcal{S^\prime}}) \leq D_j({\mathcal{S}}).
\]
Thus
\[
\Delta D = (D_i({\mathcal{S^\prime}}) + D_j({\mathcal{S^\prime}})) - (D_i({\mathcal{S}}) + D_j({\mathcal{S}})) \leq 0.
\]

%{\bf MM: I think you're stuck with this assumption;  you can put it in the theorem, and explain this shows that sorting in this way is "intuitively good"; 
%may not be perfect when this assumption is broken, but claim the assumption is rarely broken.  Maybe then provide experimental results if possible.}

\textbf{Changes in $\Delta R_i$ for Requests 
\( k \ne i, j \)}
Swapping \( i \) and \( j \) changes the cumulative memory usage profile of the system over time. By scheduling the lower-memory request \( j \) before the higher-memory request \( i \), the cumulative memory consumption at all times is the same or reduced. This can lead to reduced delays for other requests that start during or after the time interval when \( j \) and \( i \) are processed. Since the positions of other requests relative to each other remain unchanged, their waiting times \( W_k \) remain the same.

Therefore, for each \( k \ne i, j \):
\begin{align*}
\Delta R_k &= R_k(S') - R_k(S) \\
           &= [W_k(S') - W_k(S)] + [D_k(S') - D_k(S)] + (S_k - S_k) \\
           &= \Delta D_k.
\end{align*}
since \( W_k(S') = W_k(S) \) and \( S_k \) remains the same.

Our goal is to show that \( \Delta D_k \leq 0 \) for all \( k \ne i, j \).  As stated before, when we swap \( i \) and \( j \), the cumulative memory consumption at any time \( t \) becomes lower during the time when \( j \) is processed first, leading to a reduced cumulative memory usage at earlier times.
Thus, the delays for other requests \( k \ne i, j \) do not increase and may decrease due to the swap.
Accordingly,
\[
D_k(S') \leq D_k(S) \implies \Delta D_k = D_k(S') - D_k(S) \leq 0.
\]

\textbf{Total Change in Response Time.}
The total change in response time is:
\[
\Delta T_{\text{total}} = \Delta R_i + \Delta R_j + \sum_{k \ne i,j} \Delta R_k = (S_j - S_i) + (\Delta D_i + \Delta D_j) + \sum_{k \ne i,j} \Delta D_k.
\]

Since \( \Delta D_k \leq 0 \) for all \( k \ne i, j \), and \( \Delta D_i + \Delta D_j \leq 0 \), we have:

\[
\Delta T_{\text{total}} \leq (S_j - S_i) \leq 0.
\]

\end{proof}

\paragraph{A note on the theorem assumption regarding correlation.}
While we generally assume that \( M_i > M_j \) implies \( S_i \geq S_j \), it is important to note that memory consumption \( M_i \) depends on both the service time \( S_i \) and the handling strategy applied during the API call (Preserve, Swap, or Discard). Typically, requests with longer API duration are handled using the Swap or Discard strategies to free up GPU memory. In contrast, requests with shorter service times may use the Preserve strategy, keeping data in GPU memory and resulting in higher \( M_i \) but potentially lower \( S_i \). Therefore, there are rare cases where \( M_i > M_j \) but \( S_i < S_j \), such as when request \( i \) is handled by preserve and request \( j \) by swap. However, these exceptions are infrequent, and the assumption \( M_i > M_j \implies S_i \geq S_j \) generally holds in our system. Moreover, even when $\Delta S = S_j - S_i > 0$, the reduction in cumulative delay ($\Delta D$) often offsets this difference. Therefore, although the scheduling may not be perfect when the assumption is broken, it generally leads to minimized total response time in our system as shown in Section~\ref{sec:evaluation}.

\begin{comment}

Therefore:

\[
\Delta T_{\text{total}} \leq 0.
\]

Thus:
\[
\Delta T_{\text{total}} = \Delta S + [\text{Non-positive value}] \leq 0
\]

So, swapping reduces or does not increase the total response time. By applying the swapping of all pairs of adjacent requests where a higher-memory request precedes a lower-memory one, we can iteratively minimize the total response time.
\end{comment}
