# Supplementary material for: Fast Inference for Augmented Large Language Models
Source: arXiv:2410.18248 source file (2024-10-25)
Supplement: Supplementary file 2 [file appendix_evaluation.tex]

\section{Appendix}

\begin{figure*}[ht!]
    \centering
    \begin{tikzpicture}
        % Column labels
        \node at (5.5, 12) {\textbf{GPT-J 6B}};
        \node at (14.5, 12) {\textbf{Vicuna 13B}};
        
        % Row labels
        \node[rotate=90] at (1, 9) {\textbf{Single}};
        \node[rotate=90] at (1, 4) {\textbf{Multi}};
        \node[rotate=90] at (1, -1) {\textbf{ToolBench}};

        % Separator between the two columns
        \draw[dashed, gray, very thin] (10, 11) -- (10, -2);

        % Legend (adjust position as needed)
        \node at (10, -4) {
            \begin{minipage}{0.6\textwidth}
                \centering
                \includegraphics[width=\textwidth]{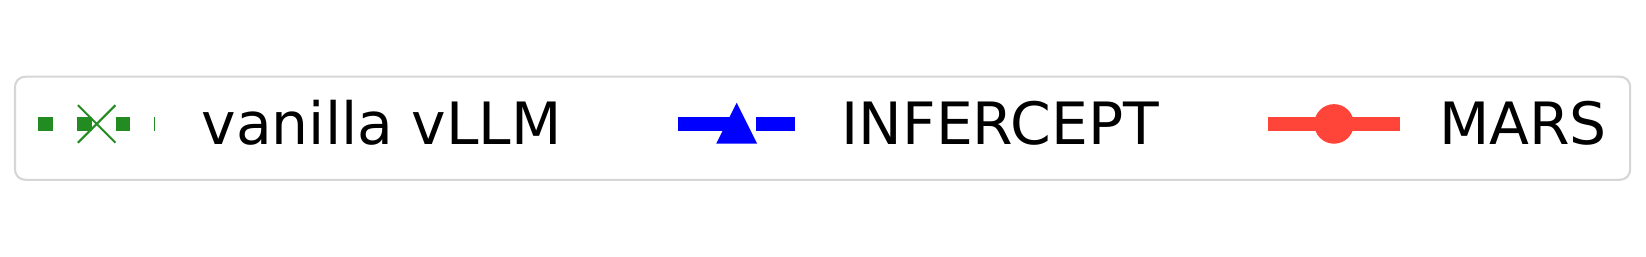}
            \end{minipage}
        };
        % First row of subfigures (Single API)
        \node at (5.5, 9) {
            \begin{minipage}{0.5\linewidth}
                \centering
                \includegraphics[width=0.3\linewidth]{eval_graphs/performance/single_api/6B/Single API_6B_1800_E2E Latency_Mean.pdf}
                \includegraphics[width=0.3\linewidth]{eval_graphs/performance/single_api/6B/Single API_6B_1800_E2E Latency_Median.pdf}
                \includegraphics[width=0.3\linewidth]{eval_graphs/performance/single_api/6B/Single API_6B_1800_E2E Latency_P99.pdf}
                \includegraphics[width=0.3\linewidth]{eval_graphs/performance/single_api/6B/Single API_6B_1800_TTFT_Mean.pdf}
                \includegraphics[width=0.3\linewidth]{eval_graphs/performance/single_api/6B/Single API_6B_1800_TTFT_Median.pdf}
                \includegraphics[width=0.3\linewidth]{eval_graphs/performance/single_api/6B/Single API_6B_1800_TTFT_P99.pdf}
            \end{minipage}
        };
        \node at (14.5, 9) {
            \begin{minipage}{0.5\linewidth}
                \centering
                \includegraphics[width=0.3\linewidth]{eval_graphs/performance/single_api/13B/Single API_13B_1800_E2E Latency_Mean.pdf}
                \includegraphics[width=0.3\linewidth]{eval_graphs/performance/single_api/13B/Single API_13B_1800_E2E Latency_Median.pdf}
                \includegraphics[width=0.3\linewidth]{eval_graphs/performance/single_api/13B/Single API_13B_1800_E2E Latency_P99.pdf}
                \includegraphics[width=0.3\linewidth]{eval_graphs/performance/single_api/13B/Single API_13B_1800_TTFT_Mean.pdf}
                \includegraphics[width=0.3\linewidth]{eval_graphs/performance/single_api/13B/Single API_13B_1800_TTFT_Median.pdf}
                \includegraphics[width=0.3\linewidth]{eval_graphs/performance/single_api/13B/Single API_13B_1800_TTFT_P99.pdf}
            \end{minipage}
        };

        % Second row of subfigures (Multi API)
        \node at (5.5, 4) {
            \begin{minipage}{0.5\linewidth}
                \centering
                \includegraphics[width=0.3\linewidth]{eval_graphs/performance/mult_api/6B/Multi API_6B_1800_E2E Latency_Mean.pdf}
                \includegraphics[width=0.3\linewidth]{eval_graphs/performance/mult_api/6B/Multi API_6B_1800_E2E Latency_Median.pdf}
                \includegraphics[width=0.3\linewidth]{eval_graphs/performance/mult_api/6B/Multi API_6B_1800_E2E Latency_P99.pdf}
                \includegraphics[width=0.3\linewidth]{eval_graphs/performance/mult_api/6B/Multi API_6B_1800_TTFT_Mean.pdf}
                \includegraphics[width=0.3\linewidth]{eval_graphs/performance/mult_api/6B/Multi API_6B_1800_TTFT_Median.pdf}
                \includegraphics[width=0.3\linewidth]{eval_graphs/performance/mult_api/6B/Multi API_6B_1800_TTFT_P99.pdf}
            \end{minipage}
        };
        \node at (14.5, 4) {
            \begin{minipage}{0.5\linewidth}
                \centering
                \includegraphics[width=0.3\linewidth]{eval_graphs/performance/mult_api/13B/Multi API_13B_1800_E2E Latency_Mean.pdf}
                \includegraphics[width=0.3\linewidth]{eval_graphs/performance/mult_api/13B/Multi API_13B_1800_E2E Latency_Median.pdf}
                \includegraphics[width=0.3\linewidth]{eval_graphs/performance/mult_api/13B/Multi API_13B_1800_E2E Latency_P99.pdf}
                \includegraphics[width=0.3\linewidth]{eval_graphs/performance/mult_api/13B/Multi API_13B_1800_TTFT_Mean.pdf}
                \includegraphics[width=0.3\linewidth]{eval_graphs/performance/mult_api/13B/Multi API_13B_1800_TTFT_Median.pdf}
                \includegraphics[width=0.3\linewidth]{eval_graphs/performance/mult_api/13B/Multi API_13B_1800_TTFT_P99.pdf}
            \end{minipage}
        };

        % Third row of subfigures (ToolBench Latency)
        \node at (5.5, -1) {
            \begin{minipage}{0.5\linewidth}
                \centering
                \includegraphics[width=0.3\linewidth]{eval_graphs/performance/toolbench/6B/Multi API_6B_1800_E2E Latency_Mean.pdf}
                \includegraphics[width=0.3\linewidth]{eval_graphs/performance/toolbench/6B/Multi API_6B_1800_E2E Latency_Median.pdf}
                \includegraphics[width=0.3\linewidth]{eval_graphs/performance/toolbench/6B/Multi API_6B_1800_E2E Latency_P99.pdf}
                \includegraphics[width=0.3\linewidth]{eval_graphs/performance/toolbench/6B/Multi API_6B_1800_TTFT_Mean.pdf}
                \includegraphics[width=0.3\linewidth]{eval_graphs/performance/toolbench/6B/Multi API_6B_1800_TTFT_Median.pdf}
                \includegraphics[width=0.3\linewidth]{eval_graphs/performance/toolbench/6B/Multi API_6B_1800_TTFT_P99.pdf}
            \end{minipage}
        };
        \node at (14.5, -1) {
            \begin{minipage}{0.5\linewidth}
                \centering
                \includegraphics[width=0.3\linewidth]{eval_graphs/performance/toolbench/13B/Multi API_13B_1800_E2E Latency_Mean.pdf}
                \includegraphics[width=0.3\linewidth]{eval_graphs/performance/toolbench/13B/Multi API_13B_1800_E2E Latency_Median.pdf}
                \includegraphics[width=0.3\linewidth]{eval_graphs/performance/toolbench/13B/Multi API_13B_1800_E2E Latency_P99.pdf}
                \includegraphics[width=0.3\linewidth]{eval_graphs/performance/toolbench/13B/Multi API_13B_1800_TTFT_Mean.pdf}
                \includegraphics[width=0.3\linewidth]{eval_graphs/performance/toolbench/13B/Multi API_13B_1800_TTFT_Median.pdf}
                \includegraphics[width=0.3\linewidth]{eval_graphs/performance/toolbench/13B/Multi API_13B_1800_TTFT_P99.pdf}
            \end{minipage}
        };
    \end{tikzpicture}
    \caption{End-to-end performance (mean, median and P99 of latency and TTFT) as a function of request arrival rate when serving GPT-J 6B and Vicuna 13B using different datasets (single-API, multi-API, ToolBench).}
\end{figure*}

\begin{comment}
    
\begin{figure}[t]
    \centering
    \begin{subfigure}[b]{0.45\linewidth}
        \centering
        \includegraphics[width=\textwidth]{eval_graphs/performance/mult_api/6B/starvation_prevension/M}
        \label{fig:err_starvation_throughput}
    \end{subfigure}
    \hfill
    \begin{subfigure}[b]{0.45\linewidth}
        \centering
        \includegraphics[width=\textwidth]{eval_graphs/performance/mult_api/6B/starvation_prevension/Multi API_6B_1800_P99_E2E Latency.pdf}
        \label{fig:err_starvation_latency}
    \end{subfigure}
    \includegraphics[width=\linewidth]{eval_graphs/performance/mult_api/6B/starvation_prevension/strategy_legend_small.pdf}
    \caption{Starvation threshold,  Multi-API dataset with GPT-J 6B.}
    \label{fig:starvation}
\end{figure}

\end{comment}

%Add starvation prevention parameters quantum
